# Supplementary material for: Exploratory Analysis of Federated Learning Methods with Differential Privacy on MIMIC-III
Source: arXiv:2302.04208 source file (2023-02-08)
Supplement: Supplementary file 1 [file List_of_figures.tex]

M3: could be seed specific
1. ho_epoch_vs_round -  
2. ho_centralized
3. he_epoch_vs_round
4. he_centralized
5. he_fedprox (all combination of epoch_vs_round)
6b.ho_dp_sgd
6a.ho_dp_sgd (Run further experiments which did not converge)
7. ho_dp_svt

CLL: (could be seed specific)
D: 1. ho_epoch_vs_round
M: 2. ho_centralized
D: 3. he_epoch_vs_round
M: 4. he_centralized
5. he_fedprox (all combination of epoch_vs_round)
6b.ho_dp_sgd
6a.ho_dp_sgd (Run further experiments which did not converge)
7. ho_dp_svt

CLL splits:
Homogeneous:
 Final_ratio: 0.9990118577075099
site1_ho_50: 0.19485657764589515
site2_ho_50: 0.1956521739130435
 Final_ratio: 0.6663920922570017
site1_ho_40: 0.19530284301606923
site2_ho_60: 0.19522240527182866
 Final_ratio: 0.42766407904022585
site1_ho_30: 0.19471947194719472
site2_ho_70: 0.19548341566690192
 Final_ratio: 0.24953675108091414
site1_ho_20: 0.19554455445544555
site2_ho_80: 0.19518221124150711
 Final_ratio: 0.11092806150466776
site1_ho_10: 0.19306930693069307
site2_ho_90: 0.19549697968149368
 Final_ratio: 0.05254942767950052
site1_ho_05: 0.19801980198019803
site2_ho_95: 0.19510926118626432

Heterogeneous splot:
 Final_ratio: 0.6666666666666666, sizes: s1: 1011, s2: 1012
site1_he_40: 0.1562809099901088
site2_he_60: 0.2341897233201581
 Final_ratio: 0.4311594202898551, sizes: s1: 1011, s2: 1012
site1_he_30: 0.11770524233432245
site2_he_70: 0.2727272727272727
 Final_ratio: 0.25, sizes: s1: 1011, s2: 1012
site1_he_20: 0.0781404549950544
site2_he_80: 0.31225296442687744
 Final_ratio: 0.11267605633802817, sizes: s1: 1011, s2: 1012
site1_he_10: 0.03956478733926805
site2_he_90: 0.35079051383399207
 Final_ratio: 0.05333333333333334, sizes: s1: 1011, s2: 1012
site1_he_05: 0.019782393669634024
site2_he_95: 0.3705533596837945
